# Supplementary material for: Mixing and de-mixing of model microswimmers in bi-motility mixtures
Source: arXiv:1709.09085 ancillary file (2017-09-26)
Supplement: Supplementary file 1 [file suppplemental_material.pdf]

# Supplemental Material
# Mixing and de-mixing of model microswimmers in bi-motility mixtures

Adyant Agrawal and Sujin B. Babu
*Department of Physics, Indian Institute of Technology, Delhi*

## I. MOVIE CAPTIONS

MOVIE 1. The movie corresponds to the simulation of system under circular confinement with radius $R = 100$ and $N_a = N_b = 75$. The green colored swimmers are faster than the red colored swimmers. $\nu_a$(green)$= 0.0065$ and $\nu_b$(red)$= 0.0035$. The arrows in the movie point towards the region where the clusters of slow swimmers near to the wall are fragmented by the fast swimmers and thus the slower ones move towards the center.

MOVIE 2. The movie corresponds to the simulation of system under circular confinement with radius $R = 100$ and $N_a = N_b = 75$. The green colored swimmers are faster than the red colored swimmers. $\nu_a$(green)$= 0.00505$ and $\nu_b$(red)$= 0.00495$. The arrows in the movie point towards the mixed clusters in which the greater number of slowers ones can be seen at the back utilizing the thrust of faster swimmers. After some time, the slower ones seggregate out of the cluster.

## II. FIGURES

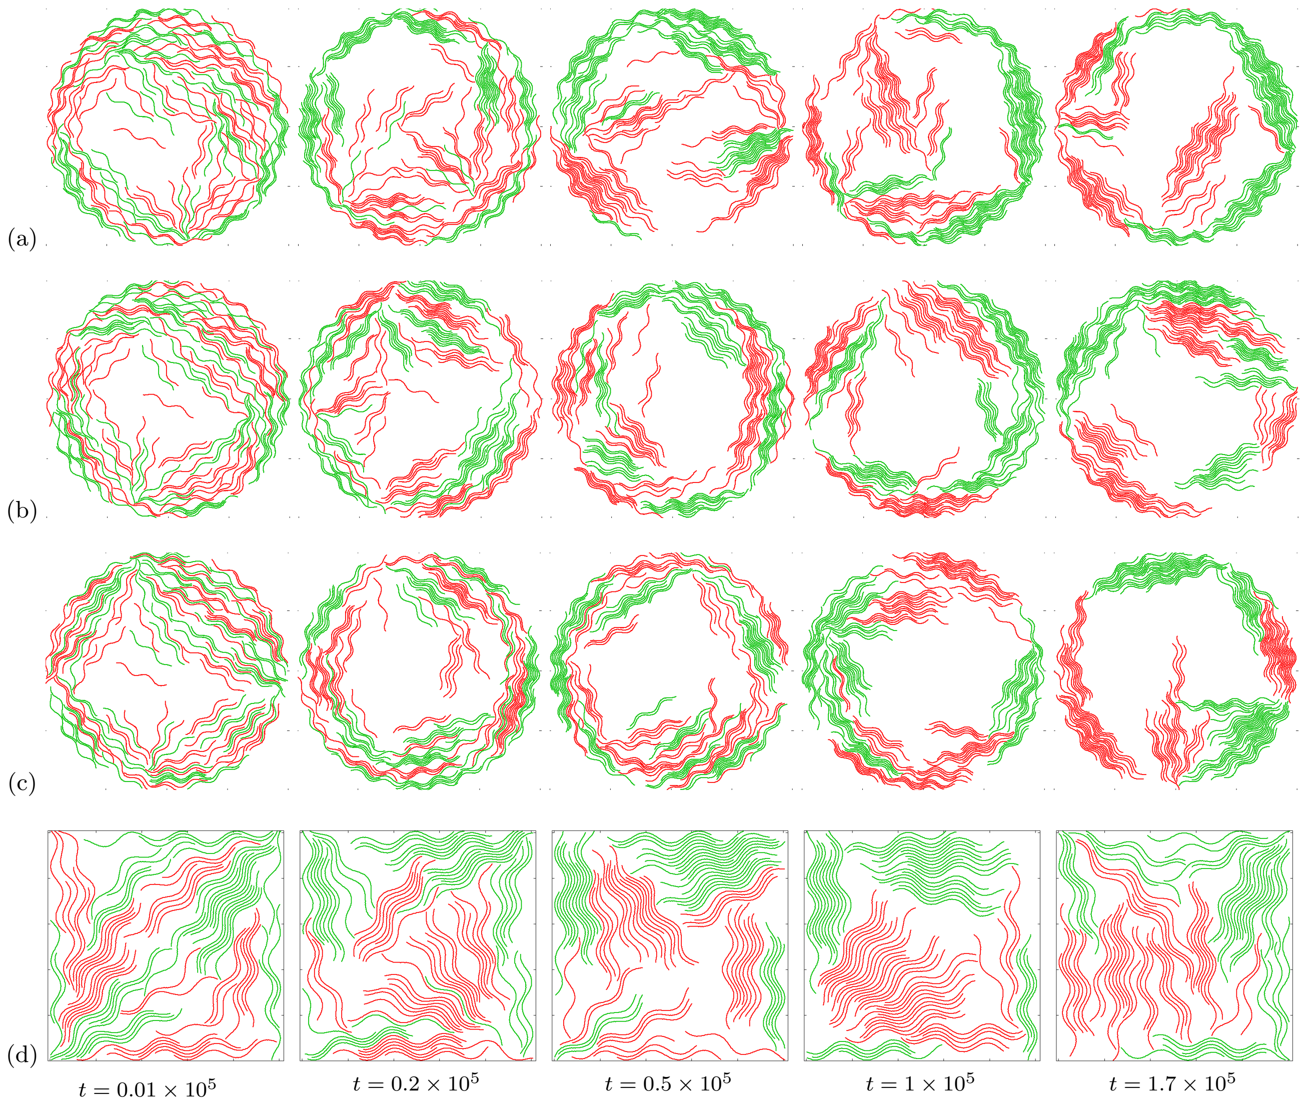


FIG. S1. Snapshots showing time evolution of 3 systems(a,b,c) under circular confinement with radius $R = 100$ and $N_a = N_b = 75$, and one system (d) under square confinement with $L = 100$ and $N_a = 37, N_b = 38$. Here green colored swimmers are faster than the red colored swimmers. For (a) $\delta\nu_a = 1.2$, (b) $\delta\nu_b = 0.2$, (c) $\delta\nu_c = 0.04$ and db $\delta\nu_d = 0.1$ . The snapshot at $t = 0.01 \times 10^5$ shows initial state where both the type of swimmer are distributed uniformly over the area. The snapshots at $t = 0.2 \times 10^5$,$t = 0.5 \times 10^5$, $t = 1 \times 10^5$ show the intermediate state before the system segregates into fast and slow swimmers. The dynamics of the system as can be observed for (a), the faster swimmers quickly reach the boundary while the slower ones are suspended near the center at the time. At intermediate $\delta\nu_b$ both kind of swimmers are able to form only small clusters due to competition between the swimmer for clustering. When the $\delta\nu_c$ is made close to zero (c) both swimmers cooperate to form big clusters and then slower ones slowly slide out of the clusters to form pure clusters as system evolves. For the case of square boundary and $\delta\nu_d = 0.1$ (d) the faster ones are stuck at the corners and slower ones form clusters near to the center. The snapshots at $t = 1.7 \times 10^5$ show the final state which is steady and segregated.

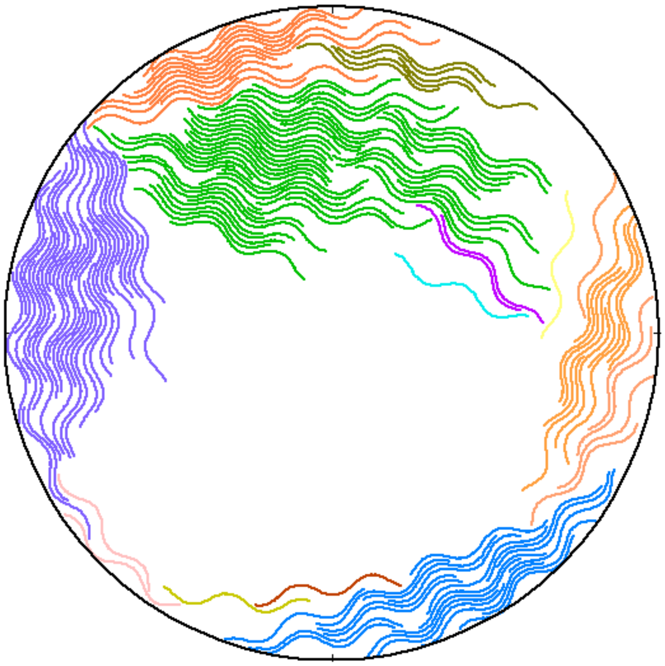

FIG. S2. Illustration showing different clusters as per our definition. Each color represents a different cluster. The snapshot is of a system with 150 swimmers in circular confinement of radius 100. The system contains homogeneous mixture of swimmers with relative difference in beating frequencies ($\delta\nu = 0.1$), $\nu_a = 0.00525$ and $\nu_b = 0.00475$. The snapshot is of the same state shown in Fig. 1a.

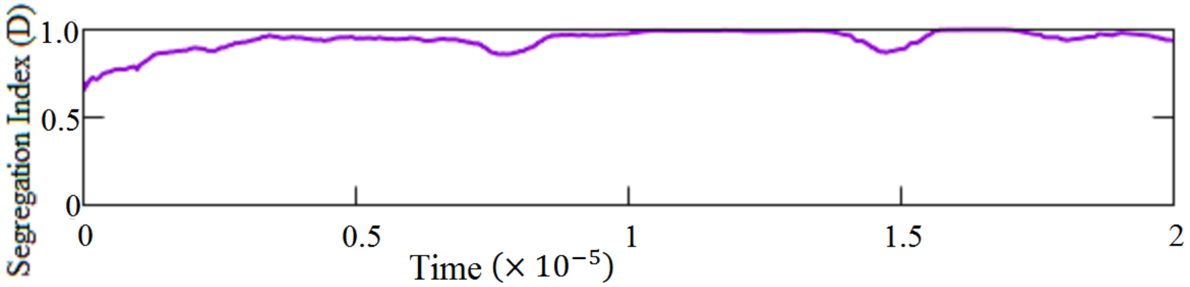


(a)

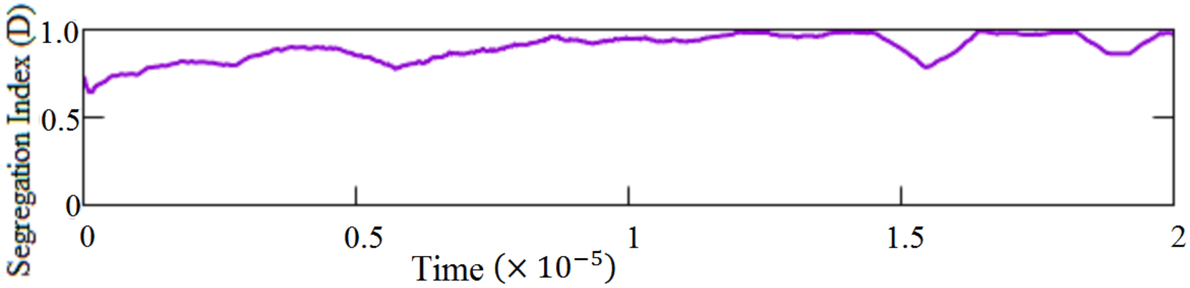


(b)

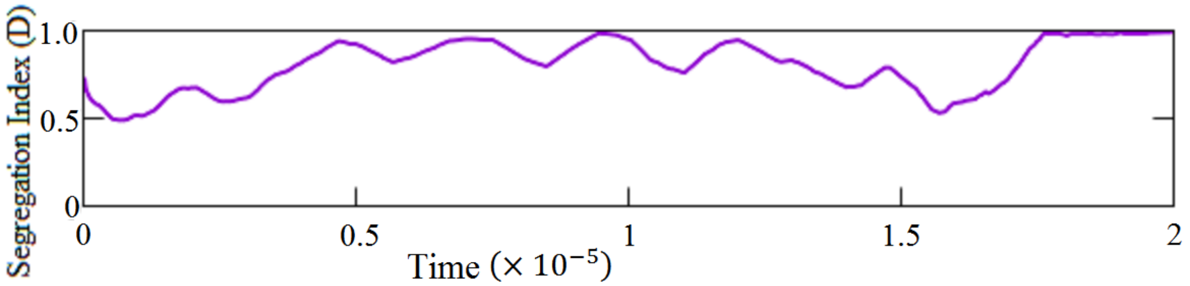


(c)

FIG. S3. Segregation Index, $D$ vs time for three systems having 150 swimmers uniformly distributed at $t = 0$ under circular confinement with $R = 100$. The systems differ in the beating frequency of swimmers, $\delta\nu_a = 0.6$, $\delta\nu_b = 0.3$ and $\delta\nu_c = 0.06$ and the average frequency in all cases is 0.005. The calculations are done for the same systems studied in Fig. 4 and in all the cases the system finally attains a segregation index close to 1 i.e. each system, regardless of $\delta\nu$ reaches a completely segregated state.
